# Supplementary material for: HiH: A Multi-modal Hierarchy in Hierarchy Network for Unconstrained Gait Recognition
Source: arXiv:2311.11210 source file (2024-05-01)
Supplement: Supplementary file 1 [file X_suppl.tex]

% \clearpage
% \setcounter{page}{1}
% \maketitlesupplementary

\appendix

\section{Supplementary Material}
\label{sec:rationale}
The supplementary material includes:
\begin{itemize}
\item The results after discarding illegal sequences for OUMVLP.
\item More detailed results for CASIA-B.
\item Cross-dataset evaluation results.
\end{itemize}

\begin{table}[htbp]
% \vspace{-5.0em}
  \centering
  \caption{Rank-1 accuracy for cross-dataset experimental settings. GREW$\longrightarrow$Gait3D denotes that the model is trained in GREW and tested in Gait3D. Gait3D$\longrightarrow$GREW denotes that the model is trained in Gait3D and tested in GREW.}
  \resizebox{0.9\linewidth}{!}{
    \begin{tabular}{c|c|c|c}
    \toprule
    \multirow{2}[4]{*}{Method} & \multirow{2}[4]{*}{Venue} & GREW$\longrightarrow$Gait3D & Gait3D$\longrightarrow$GREW \\
\cmidrule{3-4}          &       & Rank-1 & Rank-1 \\
    \midrule
    GaitSet \cite{chao2019gaitset} & AAAI19 & 19.0  & 19.2  \\
    % \midrule
    GaitPart \cite{fan2020gaitpart} & CVPR20 & 19.3  & 14.2  \\
    % \midrule
    GaitGL \cite{Lin_2021_ICCV} & ICCV21 & 15.6  & 14.3  \\
    % \midrule
    GaitBase \cite{fan2023opengait} & CVPR23 & \underline{28.9}  & 30.6  \\
    \midrule
    \rowcolor{gray!30}
    HiH-S & $-$    & \textbf{32.2}  & \textbf{36.3}  \\
    \rowcolor{gray!30}
    % \midrule
    HiH-M & $-$    & 23.8  & \underline{34.8}  \\
    \bottomrule
    \end{tabular}%
    }
  \label{tab:cross-domain}%
\end{table}%

\subsection{Details in OUMVLP}
Some probe sequences in OUMVLP do not have corresponding library sequences. The results of eliminating invalid probe sequences are shown in \cref{tab:oumvlp-probe}. Our approach achieves the best performance in all views, which reveal the generalization ability of HiH-S on large-scale datasets.
% \vspace{-1cm}
\begin{table*}[h]
  \centering
  \caption{Rank-1 accuracy (\%) on OUMVLP under all views, excluding identical-view cases and invalid probe sequences. Std denotes the performance sample standard deviation across 14 views.}
  \resizebox{1.0\linewidth}{!}{
    \begin{tabular}{c|c|cccccccccccccc|c|c}
    \toprule
    \multirow{2}[4]{*}{Method} &\multirow{2}[4]{*}{Venue} & \multicolumn{14}{c|}{Probe View}                                                                              & \multirow{2}[4]{*}{Mean} & \multirow{2}[4]{*}{Std}\\
\cmidrule{3-16}  &        & $0^{\circ}$    & $15^{\circ}$   & $30^{\circ}$   & $45^{\circ}$   &$60^{\circ}$   & $75^{\circ}$   & $90^{\circ}$   & $180^{\circ}$  & $195^{\circ}$  & $210^{\circ}$  & $225^{\circ}$  & $240^{\circ}$  & $255^{\circ}$  & $270^{\circ}$  & \\
    \midrule
    % \multicolumn{16}{c}{Excluding invalid probe sequences}\\
    \midrule
    GEINet \cite{shiraga2016geinet} &ICB16& 24.9  & 40.7  & 51.6  & 55.1  & 49.8  & 51.1  & 46.4  & 29.2  & 40.7  & 50.5  & 53.3  & 48.4  & 48.6  & 43.5  & 45.3 &8.5 \\
    GaitSet \cite{chao2019gaitset}&AAAI19 & 84.5  & 93.3  & 96.7  & 96.6  & 93.5  & 95.3  & 94.2  & 87.0  & 92.5  & 96.0  & 96.0  & 93.0  & 94.3  & 92.7  & 93.3 &3.4 \\
    GaitPart \cite{fan2020gaitpart} &CVPR20& 88.0  & 94.7  & 97.7  & 97.6  & 95.5  & 96.6  & 96.2  & 90.6  & 94.2  & 97.2  & 97.1  & 95.1  & 96.0  & 95.0  & 95.1&2.6  \\
    GLN \cite{hou2020gait} &ECCV20& 89.3  & 95.8  & 97.9  & 97.8  & 96.0  & 96.7  & 96.1  & 90.7  & 95.3  & 97.7  & 97.5  & 95.7  & 96.2  & 95.3  & 95.6 &2.5 \\
    SRN+CB \cite{hou2021set} &TBIOM21& 91.2  & 96.5  & 98.3  & 98.4  & 96.3  & 97.3  & 96.8  & 92.3  & 96.3  & 98.1  & 98.1  & 96.0  & 97.0  & 96.2  & 96.4 &2.0 \\
    GaitGL \cite{Lin_2021_ICCV}&ICCV21 & 90.5  & 96.1  & 98.0  & 98.1  & 97.0  & 97.6  & 97.1  & 94.2  & 94.9  & 97.4  & 97.4  & 95.7  & 96.5  & 95.7  & 96.2 &1.9 \\
    DyGait \cite{Wang_2023_ICCV_DyGait}&ICCV23 & \underline{96.2}  & \underline{98.2}  & \underline{99.1}  & \underline{99.0}  & \underline{98.6}  & \underline{99.0}  & \underline{98.8}  & \underline{97.9}  & \underline{97.6}  & \underline{98.8}  & \underline{98.6}  & \underline{98.1}  & \underline{98.3}  & \underline{98.2}  & \underline{98.3} &\underline{0.7} \\
    \midrule
    \rowcolor{gray!30}
    HiH-S &$-$ & \textbf{98.1}  & \textbf{99.0}  & \textbf{99.4}  & \textbf{99.5}  & \textbf{99.3}  & \textbf{99.5}  & \textbf{99.4}  & \textbf{98.9}  & \textbf{98.9}  & \textbf{99.3}  & \textbf{99.3}  & \textbf{99.0}  & \textbf{99.1}  & \textbf{99.1}  & \textbf{99.1}  &\textbf{0.3}\\
    \bottomrule
    \end{tabular}%
    }
  \label{tab:oumvlp-probe}%
  % \vspace{-0.7em}
\end{table*}%

\subsection{Details in CASIA-B}

The performance of each view for CASIA-B is shown in \cref{tab:casiab-detail}. As can be seen, our method achieves competitive performance across all viewing angles, demonstrating the superior cross-view retrieval capability of HiH-S in indoor scenes.

\begin{table*}[tbp]
  \centering
  \caption{Rank-1 accuracy (\%) on CASIA-B under all views and different conditions, excluding identical-view cases.}
  \resizebox{1.0\linewidth}{!}{
    \begin{tabular}{c|c|ccccccccccc|c}
    \toprule
    \multicolumn{2}{c|}{Gallery NM \#1-4} & \multicolumn{11}{c|}{$0^{\circ}-180^{\circ}$}                                                         & \multirow{1}[4]{*}{Mean} \\
\cline{1-13}    \multicolumn{2}{c|}{Probe} & $0^{\circ}$    & $18^{\circ}$   & $36^{\circ}$   & $54^{\circ}$   & $72^{\circ}$   & $90^{\circ}$   & $108^{\circ}$  & $126^{\circ}$  & $144^{\circ}$  & $162^{\circ}$  & $180^{\circ}$  &  \\
    \hline
    \multirow{5}[10]{*}{NM \#5-6} & GaitGraph2 \cite{teepe2022towards} & 78.5  & 82.9  & 85.8  & 85.6  & 83.1  & 81.5  & 84.3    & 83.2  & 84.2  & 81.6  & 71.8  & 82.0 \\
\cline{2-14}    & GaitSet \cite{chao2019gaitset} & 90.8  & 97.9  & \underline{99.4}  & 96.9  & 93.6  & 91.7  & 95.0    & 97.8  & 98.9  & 96.8  & 85.8  & 95.0 \\
% \cline{14-14}         & ACL   & 92.0    & 98.5  & \textbf{100.0}   & \textbf{98.9}  & 95.7  & 91.5  & 94.5  & 97.7  & 98.4  & 96.7  & 91.9  & 96.0 \\
\cline{14-14}          & GaitPart \cite{fan2020gaitpart} & 94.1  & \underline{98.6}  & 99.3  & \textbf{98.5}  & 94.0    & 92.3  & 95.9  & 98.4  & 99.2  & 97.8  & 90.4  & 96.2 \\
% \cline{14-14}          & MT3D  & 95.7  & 98.2  & 99.0    & 97.5  & 95.1  & 93.9  & 96.1  & 98.6  & 99.2  & 98.2  & 92.0    & 96.7 \\
\cline{14-14}          & GaitGL \cite{Lin_2021_ICCV} & 96.0    & 98.3  & 99.0    & 97.9  & 96.9  & 95.4  & 97.0    & 98.9  & 99.3  & 98.8  & 94.0    & 97.4 \\
\cline{14-14}          & LagrangeGait \cite{chai2022lagrange} & 95.7  & 98.1  & 99.1  & 98.3  & 96.4  & 95.2  & 97.5  & \underline{99.0}    & 99.3  & 98.9  & 94.9  & 97.5 \\
\cline{14-14}          & DANet \cite{Ma_2023_CVPR} & 96.4    & \textbf{99.1}  & 99.2    & 98.2  & 96.6  & 95.5  & \underline{97.6}    & \textbf{99.4}  & \textbf{99.5}  & \textbf{99.3}  & \underline{96.9}    & 98.0 \\
\cline{14-14}          & HSTL \cite{Wang_2023_ICCV} & \underline{97.6}  & 98.0  & \textbf{99.6}    & 98.2    & \underline{97.4}  & \textbf{96.5}  & \textbf{97.9}  & \underline{99.3}  & \underline{99.4}  & 98.4  & \textbf{97.0}  & \textbf{98.1} \\
% \rowcolor{gray!30}
\cline{2-14}          & HiH-S & \textbf{97.8}  & \textbf{99.1}  & 99.2    & \underline{98.3}    & \textbf{97.5}  & \underline{95.9}  & \textbf{97.9}  & \textbf{99.4}  & \underline{99.4}  & \underline{99.2}  & 96.4  & \textbf{98.2} \\
    \hline
    \multirow{4}[12]{*}{BG \#1-2} & GaitGraph2 \cite{teepe2022towards} & 69.9  & 75.9  & 78.1  & 79.3  & 71.4  & 71.7    & 74.3  & 76.2    & 73.2  & 73.4  & 61.7    & 73.2 \\
\cline{2-14} & GaitSet \cite{chao2019gaitset} & 83.8  & 91.2  & 91.8  & 88.8  & 83.3  & 81.0    & 84.1  & 90.0    & 92.2  & 94.4  & 79.0    & 87.2 \\
\cline{14-14}           & GaitPart \cite{fan2020gaitpart} & 89.1  & 94.8  & 96.7  & 95.1  & 88.3  & 84.9  & 89.0    & 93.5  & 96.1  & 93.8  & 85.8  & 91.5 \\
% \cline{14-14}           & MT3D  & 91.0    & 85.4  & 97.5  & 94.2  & 92.3  & 86.9  & 91.2  & 95.6  & 97.3  & 96.4  & 86.6  & 93.0 \\
\cline{14-14}          & GaitGL \cite{Lin_2021_ICCV} & 92.6  & 96.6  & 96.8  & 95.5  & 93.5  & 89.3  & 92.2  & 96.5  & 98.2  & 96.9  & 91.5  & 94.5 \\
\cline{14-14}           & LagrangeGait \cite{chai2022lagrange} & 94.2  & 96.2  & 96.8  & 95.8  & 94.3  & 89.5  & 91.7  & 96.8  & 98.0    & 97.0    & 90.9  & 94.6 \\
\cline{14-14}           & DANet \cite{Ma_2023_CVPR} & \textbf{95.0}  & \underline{97.3}  & \textbf{98.3}  & \textbf{97.4}  & \underline{94.7}  & 91.0  & 93.9  & 97.4  & 98.2  & 97.6  & \underline{94.2}  & \underline{95.9} \\
\cline{14-14}          & HSTL \cite{Wang_2023_ICCV} & \textbf{95.0}  & 96.5  & 97.3  & 96.6  & \underline{95.3}  & \textbf{93.3}  & \underline{94.6}  & 96.8  & \underline{98.6}  & \underline{97.7}  & 92.9    & \underline{95.9} \\
\cline{2-14}          & HiH-S & \underline{94.5}  & \textbf{97.5}  & \underline{97.6}  & \underline{96.8}  & \textbf{95.7}  & \underline{92.9}  & \textbf{94.8}  & \textbf{97.8}  & \textbf{98.7}  & \textbf{98.1}  & \textbf{94.6}    & \textbf{96.3} \\
    \hline
    \multirow{4}[12]{*}{CL \#1-2}& GaitGraph2 \cite{teepe2022towards} & 57.1  & 61.1  & 68.9  & 66.0  & 67.8  & 65.4  & 68.1  & 67.2  & 63.7  & 63.6  & 50.4    & 63.6 \\
\cline{2-14} & GaitSet \cite{chao2019gaitset} & 61.4  & 75.4  & 80.7  & 77.3  & 72.1  & 70.1  & 71.5  & 73.5  & 73.5  & 68.4  & 50.0    & 70.4 \\
\cline{14-14}         & GaitPart \cite{fan2020gaitpart} & 70.7  & 85.5  & 86.9  & 83.3  & 77.1  & 72.5  & 76.9  & 82.2  & 83.8  & 80.2  & 66.5  & 78.7 \\
% \cline{14-14}          & MT3D  & 76.0    & 87.6  & 89.8  & 85.0    & 81.2  & 75.7  & 81.0    & 84.5  & 85.4  & 82.2  & 68.1  & 81.5 \\
\cline{14-14}          & GaitGL \cite{Lin_2021_ICCV} & 76.6  & 90.0    & 90.3  & 87.1  & 84.5  & 79.0    & 84.1  & 87.0    & 87.3  & 84.4  & 69.5  & 83.6\\
\cline{14-14}          & LagrangeGait \cite{chai2022lagrange} & 77.4  & 90.6  & 93.2  & 90.2  & 84.7  & 80.3  & 85.2  & 87.7  & 89.3  & 86.6  & 71.0    & 85.1 \\
\cline{14-14}          & DANet \cite{Ma_2023_CVPR} & \textbf{82.8}  & \textbf{94.8}    & \textbf{96.9}  & \textbf{94.3}  & \underline{89.0}  & \underline{83.9}    & \underline{87.9}  & \underline{92.3}    & \textbf{95.1}  & \textbf{92.0}  & \textbf{80.3}  & \textbf{89.9} \\
\cline{14-14}          & HSTL \cite{Wang_2023_ICCV} & \underline{82.4}  & \underline{}{94.2}  & \underline{95.0}  & 91.7  & 88.2  & 83.3  & \textbf{88.0}  & \underline{92.3}  & \underline{93.1}  & 91.0  & \underline{78.5}  & 88.9 \\
\cline{2-14}          & HiH-S & 81.2  & 93.7  & \underline{95.0}  & \underline{92.7}  & \textbf{89.8}  & \textbf{85.2}& \textbf{88.0} &\textbf{92.7}&92.6&\underline{91.7}&78.2  & \underline{89.2} \\
    \bottomrule
    \end{tabular}%
    }
  \label{tab:casiab-detail}%
  % \vspace{-3.0em}
\end{table*}%

\subsection{Cross-dataset Evaluation}
\cref{tab:cross-domain} shows the performance of our approach and the comparison methods in a cross-dataset setting. It can be seen that HiH achieves the best rank-1 accuracy on both cross-dataset evaluations. It reveals the generality and domain-adaptability of our method.The performance of HiH-M is lower than that of HiH-S, and we conjecture that it may be due to the large bias introduced by the pose estimation, which leads to the poor generalization of the model. Finally, how to further improve the model cross-dataset performance is our next focus.
% Table generated by Excel2LaTeX from sheet 'Sheet1'
